# Supplementary material for: vid-TLDR: Training Free Token merging for Light-weight Video Transformer
Source: arXiv:2403.13347 source file (2024-03-30)
Supplement: Supplementary file 1 [file zero_shot_all.tex]

\begin{table*}[ht]
\centering
\vspace{-8pt}
\caption{
    \textbf{Comparison of zero-shot retrieval results among a baseline model~\cite{li2023unmasked}, existing token merging method (ToMe~\cite{bolya2022token}) and ours}.    
}
\vspace{-7pt}
\label{sup:zero-shot-all}
\begin{tabular}{c|c|ccc|ccc}
\thickhline

\multirow{2}{*}{} & \multirow{2}{*}{Metic} &  \multicolumn{3}{c|}{UMT-B} & \multicolumn{3}{c}{UMT-L} \\
 & & \multicolumn{1}{c}{Base} & \multicolumn{1}{c}{ToMe} & \multicolumn{1}{c|}{Ours} & \multicolumn{1}{c}{Base} & \multicolumn{1}{c}{ToMe} & \multicolumn{1}{c}{Ours} \\ \hline
 \multirow{4}{*}{Average over 4 datasets}  & GFLOPs $\downarrow$ & 78.5 & 64.7 & \textbf{48.5} & 267.8 & 179.9 & \textbf{158.7} \\
 \cline{2-8}
  & R@1  $\uparrow$ & 36.9 & 35.1 (\blue{-1.5}) & \textbf{38.0} (\red{+1.1})  & 43.7 & 42.2 (\blue{-1.5}) & \textbf{44.4} (\red{+0.7}) \\ 
  & R@5  $\uparrow$ & 61.0 & 59.2 (\blue{-1.8}) & \textbf{62.0} (\red{+1.0}) & 67.9 & 66.7 (\blue{-0.8}) & \textbf{68.4} (\red{+0.5}) \\ 
  & R@10 $\uparrow$ & 67.4 & 65.7 (\blue{-1.7}) & \textbf{68.3} (\red{+0.9}) & 73.6 & 72.6 (\blue{-1.0}) & \textbf{74.0} (\red{+0.4}) \\
  
\thickhline

\end{tabular}
\end{table*}
